# Supplementary material for: BLIP: Facilitating the Exploration of Undesirable Consequences of Digital Technologies
Source: arXiv:2405.06783 source file (2024-05-10)
Supplement: Supplementary file 1 [file 99-appendix.tex]

\newpage
\appendix

\section{The List of Aspects and Examples in BLIP}
\newcommand{\spsize}{0.12cm}

\begin{table*}[!h]
    \vskip 0.2cm
    \caption{\centering Aspects used for categorizing the \consequences of technologies along with example articles and their corresponding summaries selected from \name.}
    \label{tab:annotation}
    \Description{Table shows examples of undesirable consequences that correspond to specific codes and subcodes.}
    \centering\small
    \begin{tabular}{p{0.15cm}p{2.3cm}p{12.5cm}}
    
    \toprule

\textbf{\multirow{10}{*}[-50ex]{\rotatebox[origin=c]{90}{Aspects of Life and Society~}}} & \textsc{Health \& \newline Well-being} & It can cause motion sickness. This is due to the disconnect between what the eyes are seeing and what the body is feeling. Mayo Clinic has developed a technology that uses electrical pulses to help alleviate this problem. While this technology is still in its early stages, it has shown promise in reducing motion sickness. \newline \publisher{- Zapping Your Skull Could Alleviate Virtual-Reality Motion Sickness (MIT Technology Review)~\cite{metz_2020}}\\[\spsize]

% https://www.theverge.com/2018/1/19/16911408/vr-chat-virtual-reality-seizure
\cdashline{2-3}[1.5pt/5pt]\noalign{\vskip \spsize}
% \midrule
% health, healthcare, mental health, dopamine, addiction, social comparison, detoxing, unplugging, strain, pain, body aches

& \textsc{Security \& Privacy}
& They can easily pick up conversations from anywhere in the room, even with my wife and kids. And once hooked, the companies want us to place their mics in every room of the house. It all sounds so ominous. \newline \publisher{- First Click: Do you trust Google to always be listening inside your Home? (The Verge) ~\cite{ricker_2016}}\\[\spsize] 
% privacy, safety, security, targeting, data collection
\cdashline{2-3}[1.5pt/5pt]\noalign{\vskip \spsize}

& \textsc{Equality \& Justice} & They reinforce harmful gender stereotypes. The report argues that by naming voice assistants with traditionally female names, like Alexa and Siri, and rendering the voices as female-sounding by default, tech companies have already preconditioned users to fall back upon antiquated and harmful perceptions of women. \newline \publisher{- \emph{AI voice assistants reinforce harmful gender stereotypes, new UN report says (The Verge)}~\cite{statt_2019}}\\[\spsize] %gender bias, racial bias, bias, equality, social justice (S: discrimination, stereotypes, prejudice)
\cdashline{2-3}[1.5pt/5pt]\noalign{\vskip \spsize}

& \textsc{User Experience, Home \& Work Life Entertainment} & 
People get so immersed in the experience that they forget their surroundings. This can lead to people accidentally hurting themselves if they're not careful. \newline \publisher{- Oculus Rift Plus Motion Controls Make Shooting Almost Too Realistic~\cite{rigney_2013}}\\[\spsize]
\cdashline{2-3}[1.5pt/5pt]\noalign{\vskip \spsize}

& \textsc{Economy} & People are losing their jobs. The technology is becoming so realistic that many people can't tell the difference. \newline \publisher{- AI voice actors sound more human than ever—and they’re ready to hire (MIT Technology Review)~\cite{hao_2021}}\\[\spsize] % economy, money, financial loss, expenditures, jobs 
\cdashline{2-3}[1.5pt/5pt]\noalign{\vskip \spsize}

& \textsc{Access to Information, Discourse \& Governance} &  They have difficulty understanding natural human speech, and often produce inaccurate, inappropriate, or offensive responses as a result. Additionally, these systems often contain sexist, racist, or other offensive content due to the vast amounts of data they are trained on, which often come from the internet. \newline \publisher{- Google Has a Plan to Stop Its New AI From Being Dirty and Rude (WIRED)~\cite{simonite_2022}}\\[\spsize]

%information, governance, toxicity, conspiracy, misinformation, filter bubble, content moderation, extremism, deepfa
\cdashline{2-3}[1.5pt/5pt]\noalign{\vskip \spsize}

& \textsc{Environment \& \newline Sustainability} & They require a lot of resources to build and operate, and these resources are often extracted from developing countries with little regulation. This can lead to social and environmental problems, such as child labor and deforestation. \newline \publisher{- This beautiful map shows everything that powers an Amazon Echo, from data mines to lakes of lithium (The Verge) ~\cite{vincent_2018}}\\[\spsize]

%  the way in which they extract value from human users in the form of data, feedback, and labor, without the users being fully aware of it. This value is then concentrated in the hands of a few companies and individuals, exacerbating inequality.

% ``The concern is that machine-learning algorithms in general are consuming more and more energy, using more data, training for longer and longer,” ... It’s not just a worry for academics. As more companies across more industries begin to use AI, there’s growing fear that the technology will only deepen the climate crisis.''  %environment, sustainability, unsustainable, climate, trash, 
\cdashline{2-3}[1.5pt/5pt]\noalign{\vskip \spsize}

& \textsc{Politics} &  It can be used to manipulate public opinion. This is because social media platforms like Facebook collect a lot of data about their users, which can then be used to target them with personalized messages. In the case of Cambridge Analytica, this data was collected without users' knowledge or consent, and was then used to support the Trump election campaign. \newline \publisher{- \emph{Facebook suspends the Trump campaign’s data-mining firm amid revelations of a major data breach (MIT Technology Review)} ~\cite{giles_2022}}\\[\spsize] %politics, election, interference, censoring

% They are sometimes perceived as biased or having a political agenda. https://www.theverge.com/2020/6/8/21284546/apple-siri-amazon-alexa-google-assisant-black-lives-matter-ai-response
\cdashline{2-3}[1.5pt/5pt]\noalign{\vskip \spsize}

& \textsc{Power} & It can lead to people feeling like they are being sexually assaulted. This is because people are not limited by physical boundaries in VR, so they can get very close to each other and simulate rape. To prevent this, Facebook has rolled out a new "Personal Boundary" feature that creates a bubble of space with a radius of two virtual feet around. \newline \publisher{- Meta to allow Horizon Worlds users to turn their avatar’s personal safety boundary off (TechCrunch)~\cite{perez_2022}}\\[\spsize] % bullying, sexual assault, exploitation, predatory, vulnerable, consent, vandalism
\cdashline{2-3}[1.5pt/5pt]\noalign{\vskip \spsize}

& \textsc{Social Norms \& \newline Relationships} &  The devaluation of human interaction, social relationships and friendships. Because of our constant need for more and more information, and constant need for more and more content, we share more and more with more and more people. We've also de-personalized our relationships and have taken on a very impersonal tone with our online friends. In effect, we are creating a digital world where we are our own audience, rather than a world where we can interact with others.\newline \publisher{- The Quagmire of Social Media Friendships (WIRED)~\cite{staff_2012}}
\\[\spsize] %social norms, habits, culture, behavior, relationship, family, friends, interaction between people, roles, sexual relationship

    \bottomrule
    \end{tabular}
\end{table*}

\section{Annotation Codebook}
Two annotators qualitatively coded the relevant articles following a code book, which we developed to enable further classifications and analyses. More precisely, two authors developed an initial set of codes by independently going through all articles they individually deemed relevant to look for similarities and differences across the paragraphs. They then discussed the codes, which included \texttt{framing} that was used to describe the \consequence, the specificity of the discussion, and the aspect of life, society, or the environment that the technology influences. To develop subcodes, we used affinity diagramming to cluster articles into groups that describe similar \consequences. We started with a list of 21 aspects of life that are commonly influenced by technology (provided by the Artefact group's Tarot Cards of Tech project~\cite{TarotCardofTech}) to inform these categories. Note that in some cases, articles of \consequences may sometimes fit into two categories.  

\begin{figure}[h]
    \centering
    \includegraphics[width=\linewidth]{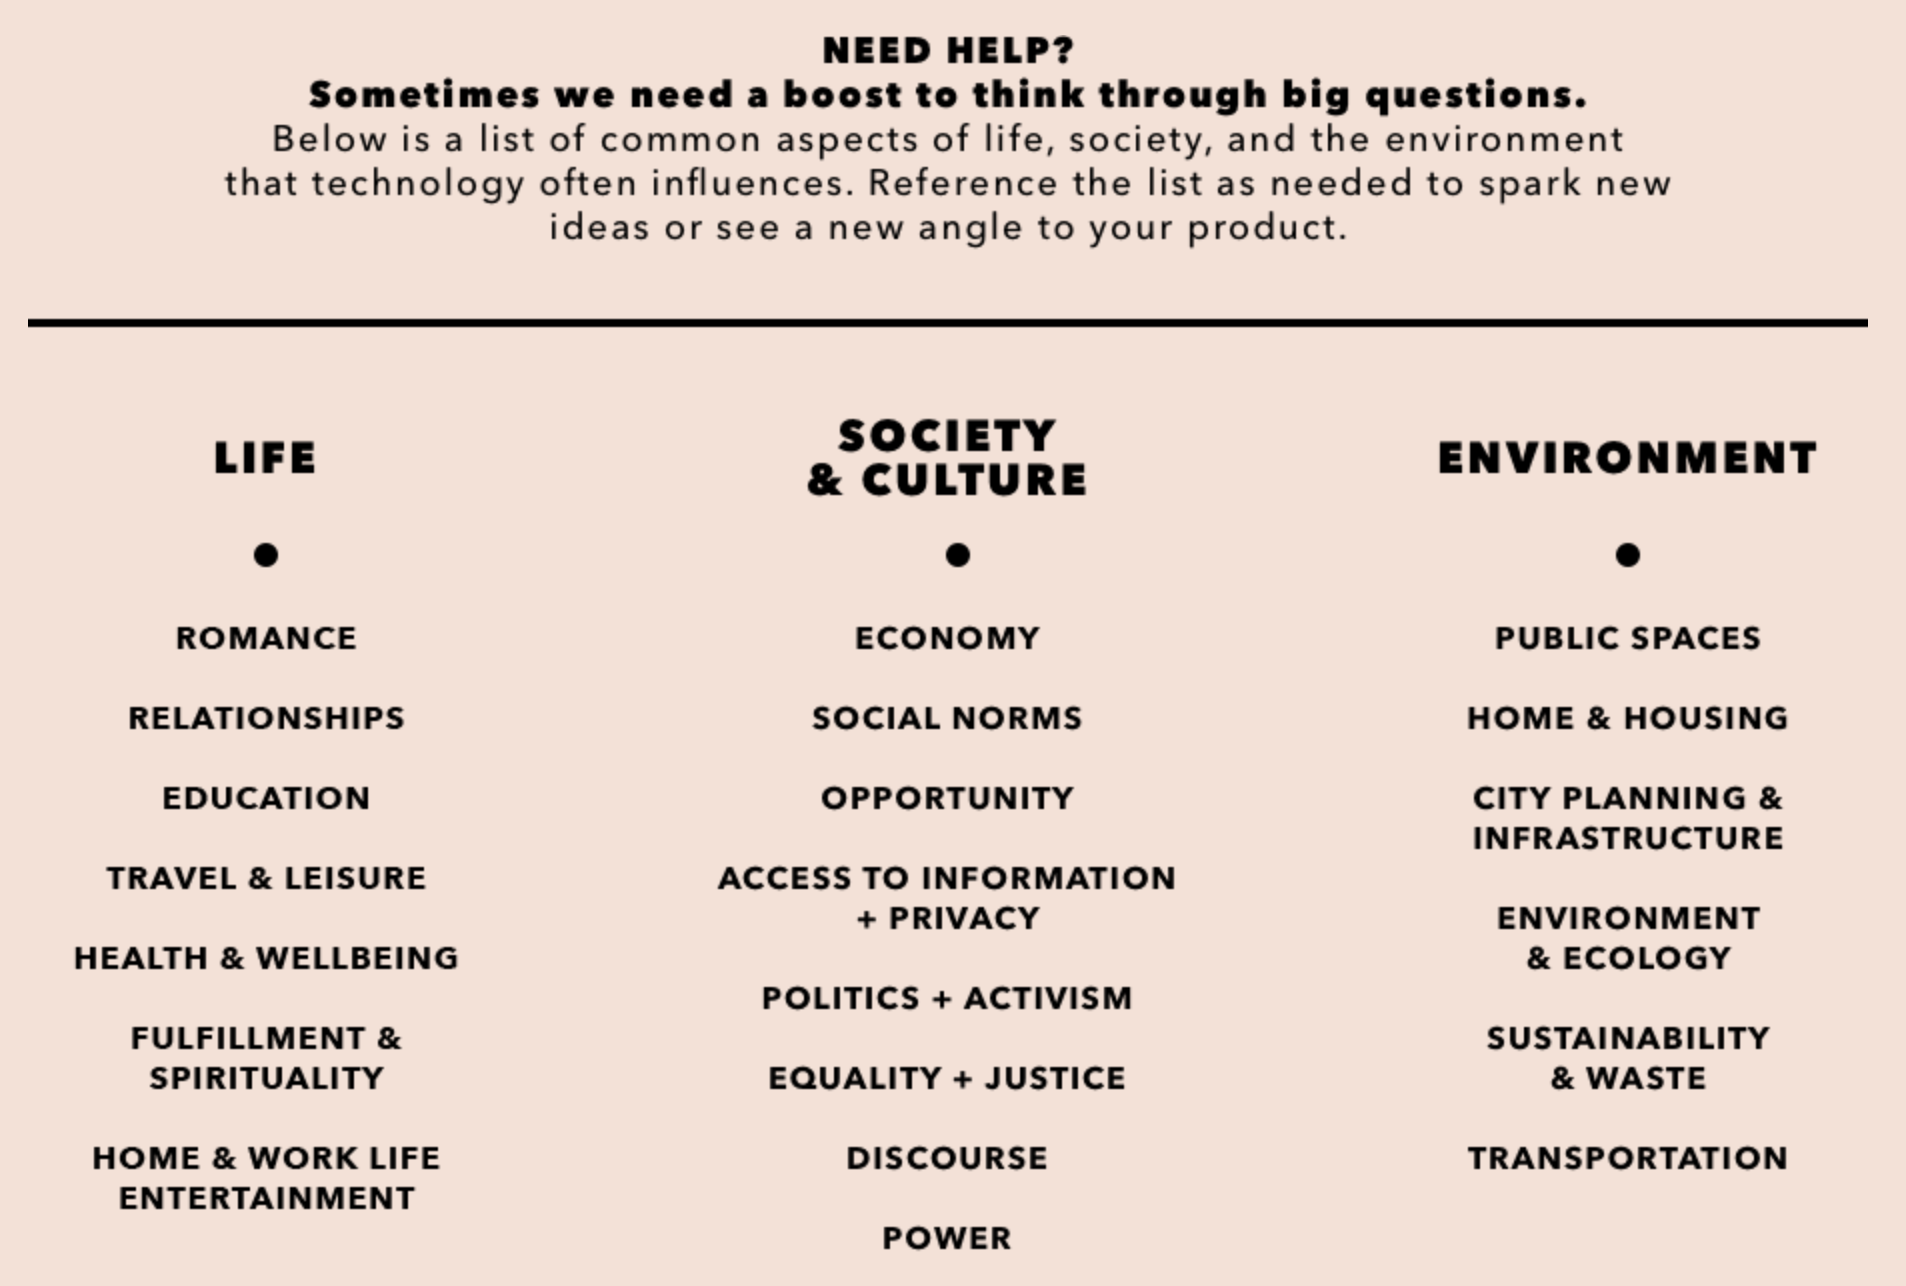}
    \caption{Aspects of Life, Society and Environment from Tarot Cards of Tech}
    \label{fig:aspects_tarot_cards}
\end{figure}

\section{NLI-based technique (previous)}
Our previous classifiers used an existing pre-trained language model fine-tuned on a Natural Language Inference (NLI) task \cite{yin2019benchmarking}.
Natural Language Inference (NLI) is a task to predict whether a given hypothesis is true (\emph{entailment}), false (\emph{contradiction}), or undetermined (\emph{neutral}) to a given  premise~\cite{yin2019benchmarking}. In our case, we use the hypothesis ``This is an example of \emph{X}'' and apply it to each sentence (each of which constitute a premise) to calculate the likelihood that the hypothesis is true or false. For example, given the premise ``Study of YouTube comments finds evidence of radicalization effect'' and the hypothesis  ``This is an example of \emph{a consequence of technology}'', our classifier returns a higher score for \emph{entailment} compared to \emph{contradiction}. Our algorithms then label any sentence returned as \emph{entailment} as an undesirable consequence. This approach has been termed as zero-shot as it does not require any further training of the pre-trained (+ NLI fine-tuned) model---however, we hand-crafted our labels to improve performance. Our choice of fine-tuned RoBERTa model for the title classifer and GPT-3 in aspect classifier yield higher precision, recall, F1 and accuracy scores.

%  \begin{table}[h]
%   \caption{Performance of Filters}
%  \label{tab:perffilter}
%  \Description{Table contains six columns with the headers Relevance Classifier, Labels, Precision, Recall, F1, and Accuracy. The maximum precision is 0.68, the maximum recall is 0.97, and the maximum F1 score and Accuracy are 0.77 and 0.64, respectively.}
%  \small
%  \begin{tabular}{lcccc}
%  \toprule
%  \textbf{Title Classifier} & \textbf{Prec.} & \textbf{Rec.} & \textbf{F1} & \textbf{Acc.} \\
%  \midrule
%  Title [always irrelevant] & 0.00 & 0.00 & 0.00 & 0.61
% \\[0.07cm]
% \hdashline[1.5pt/5pt]\noalign{\vskip 0.07cm}
% NLI (zero-shot) & 0.52 & 0.37 & 0.43 & 0.62 \\
% RoBERTa (supervised) & \textbf{0.87} & \textbf{0.86} & \textbf{0.87} & \textbf{0.87} \\
% \bottomrule
%  \end{tabular}
%  \end{table}

 \begin{table}[h]
  \caption{Performance of Filters}
 \label{tab:perffilter}
 \Description{Table contains six columns with the headers Relevance Classifier, Labels, Precision, Recall, F1, and Accuracy. The maximum precision is 0.68, the maximum recall is 0.97, and the maximum F1 score and Accuracy are 0.77 and 0.64, respectively.}
 \small
 \begin{tabular}{lcc}
 \toprule
 \textbf{Relevance Classifier} & \textbf{F1} & \textbf{Acc.} \\
 \midrule
 Title [always irrelevant] & 0.00 & 0.61
\\[0.07cm]
\hdashline[1.5pt/5pt]\noalign{\vskip 0.07cm}
NLI (zero-shot) & 0.43 & 0.62 \\
RoBERTa (supervised) & 0.87 & 0.87 \\
\textbf{gpt-3.5-turbo (zero-shot, ours)} & \textbf{0.90} & \textbf{0.89} \\
\bottomrule
 \end{tabular}
 \end{table}
% \input{sections/tables/perf-summ}
%  \begin{table}[h]
%   \caption{Performance of Aspect Classifiers}
% \label{tab:perfaspect}
%  \small
%  \begin{tabular}{lcccc}
%  \toprule
%  \textbf{Attribute Classifier} & \textbf{Prec.} & \textbf{Rec.} & \textbf{F1} & \textbf{Acc.} \\
%  \midrule
% Random & 0.09 & 0.11 & 0.09 & 0.11 \\
% \hdashline[1.5pt/5pt]\noalign{\vskip 0.07cm}
% NLI (zero-shot) & 0.31 & 0.34 & 0.30 & 0.36 \\
% \textbf{GPT-3 (zero-shot, ours)} & \textbf{0.38} & \textbf{0.34} & \textbf{0.36} & \textbf{0.38} \\
% \bottomrule
%  \end{tabular}
%  \end{table}

 \begin{table}[h]
  \caption{Performance of Aspect Classifiers}
\label{tab:perfaspect}
 \small
 \begin{tabular}{lcc}
 \toprule
 \textbf{Attribute Classifier} & \textbf{F1} & \textbf{Acc.} \\
 \midrule
Random & 0.09 & 0.11 \\
\hdashline[1.5pt/5pt]\noalign{\vskip 0.07cm}
NLI (zero-shot) & 0.30 & 0.36 \\
\textbf{gpt-3.5-turbo (zero-shot, ours)} & \textbf{0.36} & \textbf{0.38} \\
\bottomrule
 \end{tabular}
 \end{table}

\section{Study 2: Participants information and responses}
\label{study_2}

%Table with participants, their research area, their prior ethics exposure (or whether they work on societal impacts), a rough description of their project, and then the UCs they came up with (maybe example ones)
\FloatBarrier
\begin{table*}[h!]
\centering
\caption{Study 2 participants, their areas, and example  undesirable consequences they bookmarked as relevant to their own projects.}
\label{table:research_participants}
\begin{tabular}{p{0.02\linewidth}|p{2.0cm}|p{0.9\linewidth}}
\toprule
ID & Research Area & Example Consequence Derived From \name \\
\hline
\hline
P1 & Computer Vision & (1) Pretrained vision models risk not obtaining consent from users especially children; (2) CV projects in AR environmet might distract people; (3) Google Glass head-tilt-to-wake function caused traffic accident and had legal consequences; (4) bias in the pretrained models in identifying potential objects, especially in countries not in the training data \\
\hline
P2 & Vision Language Models & (1) Listening-based back navigation can be time-consuming and cognitively taxing as users need listen to each previous page to retrieve desired content; (2) The increasing reliance on voice assistants like Alexa may lead to a decrease in customization and creativity; (3) vision language models can struggle with identifying minority groups; (4) Facial expressions can interrupt responses from smart speakers, where misunderstandings of users' requests can lead to dangerous responses; (5) voice assistants are recording everything we say; (6) ``Echo chamber'' effect where models are pre-programmed with certain political agenda; (7) Severe privacy issues in smart homes devices; (8) Effects on non-native speakers' comprehension in real-time computer-mediated communication; (9) The Pentagon's blue-sky researchers funded a project that uses crowdsourcing to improve how machines analyze our speech -- and let you easily record, transcribe and recall all the conversations you ever have; (10) Conversational cues when interacting with voice assistants can lead to a lack of transparency and accountability in the decision-making process; (11)voice assistants can be used to make fraudulent payments or access sensitive information without user's consent; (12) Verbal abuses toward conversational agents can in turn affect users' emotion.
\\
\hline
P3 & Mobile Technologies & (1) Smart phones can tell if you're bored and then manipulate users' emotions in a negative way; (2) Facial expressions can interrupt responses from mobile smart speakers, where misunderstandings of users' requests can lead to dangerous responses; (3) Small, easily accessible, and discreet wearable input could positively impact the ability of people with visual impairments to access information on the go; (4) AI voice assistants sound more human and people are losing jobs because of that; (5) US Army soldiers will soon wear Microsoft's HoloLens AR goggles in combat \\
\hline
P4 & Computational Biology & (1) High cost of discovering new drugs;  (2) production of autoantibodies that taget parts of the body the system is designed to protect can lead to autoimmune diseases. This phenomenon is seen in patients with severe COVID; (3) AI-Powered biotech can help deploy a vaccine in record time; (4) The AI-powered Computation Biology can be biased if the data to train them is biased in some ways.; (5) There is a risk of oversimplifying complex biological processes by focusing solely on genomics \\
\hline
P5 & Robotics & (1) Technical challenges of building bipedal robots due to the limitations of current motors compared to human muscles; (2) You can order a bubble tea by drone in Shenzhen, but there is a lack of control over the delivery of products; (3) There is a security concern about connecting an autonomous car to the internet, as it can be hacked; but the article proposes a solution to these \consequence that lets insurers control the cars; (4) San Francisco's restrictions on multi-wheeled delivery bots could limit the potential benefits of robotic delivery services, such as reduced traffic congestion and increased efficiency; (5) The automation of jobs brought by Robotics technology may increase inequality within societies and further entrench the divide between rich and poor; (6) People have a tendency to anthropomorphize robots, which can lead to unrealistic expectations and potential disappointment with the technology's capabilities; (7) The proposal to classify working robots as "electronic persons" and require their owners to pay social security on their behalf may stunt the development of robotics and be bureaucratic; (8) iPhone manufacturer Foxconn plans to replace almost every human worker with robots; (9) AI systems don't truly understand their tasks or the world around them; the perpectuation of discimination in deep learning algorithms may further manifest in the robotics applications\\
\hline
P6 & Ubiquitous Computing & (1) General limitation of current wearable devices, specifically their lack of accuracy when users are mobile or performing physical activity; (2) ECG biometrics, a technology used for user identification, is less robust in real-life deployments compared to lab studies, with high error rates due to noise from changing body postures and states; (3) Smart homes can monitor our vital signs such as breathing and heart rate; (4) Sensing technologies can enable emotion tracking to promote behavioral changes; (5) Ubiquitous computing systems can tell if you're depressed and infringe on your privacy to collect your emotion information. \\

\hline
\hline
\end{tabular}
\end{table*}
\FloatBarrier
